# Supplementary material for: Virtual Linking Bids for Market Clearing with Non-Merchant Storage
Source: arXiv:2309.14787 source file (2025-05-02)
Supplement: Supplementary file 1 [file appendix.tex]

First, we give an equivalent formulation of the model where the state of energy is replaced, using that $e\up{a}_t = \sum_{i=1}^{t} p_i\up{C,a}$ and $e\up{e}_{vt} = E\up{init}_v - \sum_{i=1}^{t} p_{vi}\up{D,e}$.
We also notice that in \eqref{eq:stor_pos}, $e\up{e}_{vt}\geq 0$ can be equivalently replaced by $e\up{e}_{vT}\geq 0$, since the update quantities $p_{vt}\up{D,e}$ are non-negative.
Lastly, to lighten the notations we assume that $\Delta t = 1$. The same proof can be made for any value of $\Delta t$.
We obtain the following:
\begin{subequations} \label{prob:mc_vos_proof}
\allowdisplaybreaks
\begin{alignat}{3}
    \label{eq:mc_obj_pf} \max_{\mathbf{x}} \quad & \sum_{t \in \mathcal{T}}  \left ( \sum_{l \in \mathcal{L}} U_{lt} d_{lt} - \sum_{g \in \mathcal{G}} C_{gt} p_{gt} - \sum_{v \in \mathcal{V}} S_v p_{vt}\up{D,e}  \right )\\
    \label{eq:energy_bal_pf} \text{s.t.} \quad & \sum_{l \in \mathcal{L}} d_{lt} + p_t\up{C,a} - \sum_{g \in \mathcal{G}} p_{gt}  - \sum_{v \in \mathcal{V}} p_{vt}\up{D,e} = 0 , \hspace{-0.01\linewidth} \forall t \in \mathcal{T} \\
    \label{eq:gen_bound_pf} & 0 \leq p_{gt} \leq \overline{P}_{gt}, \hspace{0.29\linewidth} \forall g \in \mathcal{G}, t \in \mathcal{T} \\
    \label{eq:load_bound_pf} & 0 \leq d_{lt} \leq \overline{D}_{lt}, \hspace{0.29\linewidth} \forall l \in \mathcal{L}, t \in \mathcal{T} \\
    \label{eq:stor_intra_lower_end_pf} & \sum_{i=1}^{T} p_i\up{C,a} \geq 0,\\
    \nonumber  & 0 \leq \sum_{i=1}^{t} p_i\up{C,a} + \sum_{v \in \mathcal{V}} \left ( E\up{init}_v - \sum_{i=1}^{t} p_{vi}\up{D,e} \right ) \leq \overline{E}, \\
    \label{eq:stor_bound_all_pf} & \hspace{0.67\linewidth}  \forall t \in \mathcal{T} \\
    \label{eq:stor_p_pf} & p_{vt}\up{D,e} \geq 0, \hspace{0.36\linewidth} \forall v \in \mathcal{V}, \,  \forall t \in \mathcal{T}\\
    \label{eq:stor_e_pf} & E\up{init}_v - \sum_{i=1}^{T} p_{vi}\up{D,e} \geq 0, \hspace{0.3\linewidth} \forall v \in \mathcal{V}\\
    \label{eq:stor_end_all_pf} & \sum_{i=1}^{T} p_i\up{C,a} + \sum_{v \in \mathcal{V}}  \left ( E\up{init}_v - \sum_{i=1}^{T} p_{vi}\up{D,e} \right ) \geq E\up{end} .
\end{alignat}
\end{subequations}

Assuming that \eqref{prob:mc_vos_proof} has feasible solutions, we consider $\mathbf{x}^*$ an optimal solution such that $\exists \, \tau \in \mathcal{T}$ with $p_\tau\up{C,a*} > 0$ and $\sum_{v \in \mathcal{V}} p_{v\tau}\up{D,e*} > 0$.
We introduce $q_v^\tau$ such that $q_v^\tau = p_{v\tau}\up{D,e*}$, and $q^\tau$ such that $q^\tau = \sum_{v \in \mathcal{V}} q_v^\tau$.
We identify $\kappa \in \mathcal{T}$ such that $p_\kappa\up{C,a*} < 0$. 

\paragraph{Existence of $\kappa$}

%We first prove that $\kappa$ exists. 
Let's suppose that $\kappa$ does not exist, i.e., that $p_t\up{C,a*} \geq 0$, $\forall t \in \mathcal{T}$. We have $\sum_{i=1}^{T} p_i\up{C,a*} > 0$ since $p_\tau\up{C,a*} > 0$.
We build a new solution $\mathbf{x}'$ that is identical to the previous solution, except for $p_\tau\up{C,a'} = p_\tau\up{C,a*} - q^{\tau'} $ and $p_{v\tau}\up{D,e'} = p_{v\tau}\up{D,e*} - q_v^{\tau'}$, $\forall v \in \mathcal{V}$, with $q^{\tau'} = \min \{q^{\tau}, \sum_{i=1}^{T} p_i\up{C,a*}\}$ and $q_v^{\tau'}$ are such that $q^{\tau'}= \sum_{v \in \mathcal{V}} q_v^{\tau'}$ and $0 \leq q_v^{\tau'} \leq q_v^{\tau}$, $\forall v \in \mathcal{V}$. It is possible to find such $q_v^{\tau'}$, since $\sum_{i=1}^{T} p_i\up{C,a*} > 0$ and $q^{\tau} > 0$, so $0 < q^{\tau'} \leq q^{\tau}$, meaning that $0 < \sum_{v \in \mathcal{V}} q_v^{\tau'} \leq \sum_{v \in \mathcal{V}} q_v^{\tau}$.

We check that this new solution is feasible.
Constraints \eqref{eq:gen_bound_pf} and \eqref{eq:load_bound_pf} still hold.
Constraint \eqref{eq:energy_bal_pf}, at $t=\tau$, constraint \eqref{eq:stor_bound_all_pf}, with $t \geq \tau$ and constraint \eqref{eq:stor_end_all_pf} sum up to the same quantities as for $\mathbf{x}^*$, and are therefore satisfied.
For constraint \eqref{eq:stor_intra_lower_end_pf}: 
\begin{align}
    \sum_{i=1}^{T} p_i\up{C,a'} =  \sum_{i=1}^{T} p_i\up{C,a*} - q^{\tau'},
\end{align}
which we know is positive, since $q^{\tau'} = \min \{q^{\tau}, \sum_{i=1}^{T} p_i\up{C,a*}\}$.
Constraint \eqref{eq:stor_p_pf} is satisfied at $t = \tau$ since $q_v^{\tau'} \leq q_v^{\tau}$.
Constraint \eqref{eq:stor_e_pf} still holds, since we discharge less.
We can conclude that our new solution is feasible.

The value of the objective function for this solution is
\begin{align}
    \sum_{t \in \mathcal{T}}  \left ( \sum_{l \in \mathcal{L}} U_{lt} d_{lt}^{*} - \sum_{g \in \mathcal{G}} C_{gt} p_{gt}^{*}  - \sum_{v \in \mathcal{V}} S_v p_{vi}\up{D,e*} \right ) + \sum_{v \in \mathcal{V}} S_v q_v^{\tau'}.
\end{align}
We have $\sum_{v \in \mathcal{V}} S_v q_v^{\tau'} > 0 $, under the assumption that $S_v > 0$, $\forall v \in \mathcal{V}$, and since $q_v^{\tau'} \geq 0 $ , $\forall v \in \mathcal{V}$, and $\sum_{v \in \mathcal{V}} q_v^{\tau'} > 0$, meaning that there is at least one $v$ for which $q_v^{\tau'} > 0 $.
It is greater than the value of the objective function for $\mathbf{x}^*$, which is optimal, indicating a contradiction.

\textit{Note 1:} This also excludes the case where $|\mathcal{T}|=1$, meaning that it is not optimal to have $p_\tau\up{C,a*} > 0$ and $p_\tau\up{D,e*} > 0$ then.

\textit{Note 2:} $\sum_{i=1}^{T} p_i\up{C,a*} > 0$ also in case of net charge, so there will not be simultaneous charge of intra-storage and discharge of inter-storage then. 

\paragraph{Building a new solution}

%We now know that 
There exists $\kappa \in \mathcal{T}$, $\kappa \neq \tau$, such that $p_\kappa\up{C,a*} < 0$. We build a new solution $\mathbf{x}'$ to \eqref{prob:mc_vos_proof}.
It is identical to the previous solution, except that we want to discharge less the inter-storage at $t=\tau$ and discharge it more at $t=\kappa$, and in turn charge less the intra-storage at $t=\tau$ and discharge it less at $t=\kappa$, in order to keep the same storage level when both are summed. 

For $t=\tau$, $p_\tau\up{C,a'} = p_\tau\up{C,a*} - q^{\tau'}$ and $p_{v\tau}\up{D,e'} = p_{v\tau}\up{D,e*} - q_v^{\tau'}$, $\forall v \in \mathcal{V}$, with $q^{\tau'} = \min \{q^{\tau}, -p_\kappa\up{C,a*}\}$ and $q_v^{\tau'}$ are such that $q^{\tau'}= \sum_{v \in \mathcal{V}} q_v^{\tau'}$ and $0 \leq q_v^{\tau'} \leq q_v^{\tau}$, $\forall v \in \mathcal{V}$. It is possible to find such $q_v^{\tau'}$, since $-p_\kappa\up{C,a*} > 0$ and $q^{\tau} > 0$, so $0 < q^{\tau'} \leq q^{\tau}$, meaning that $0 < \sum_{v \in \mathcal{V}} q_v^{\tau'} \leq \sum_{v \in \mathcal{V}} q_v^{\tau}$.
For $t=\kappa$, $p_\kappa\up{C,a'} = p_\kappa\up{C,a*} + q^{\tau'}$ and $p_{v\kappa}\up{D,e'} = p_{v\kappa}\up{D,e*} + q_v^{\tau'}$, $\forall v \in \mathcal{V}$. 
Let's check that this solution is feasible.
Constraints \eqref{eq:gen_bound_pf} and \eqref{eq:load_bound_pf} still hold, since the solution is not modified for these variables.
For \eqref{eq:energy_bal_pf}, at $t=\tau$, and at $t=\kappa$, we have the same as for $\mathbf{x}^*$, which is feasible.
The total charged quantity in the intra-storage and the total quantity discharged from the inter-storage are unchanged. As a consequence, constraints \eqref{eq:stor_intra_lower_end_pf}, \eqref{eq:stor_e_pf} and \eqref{eq:stor_end_all_pf} are satisfied by the new solution.
Constraint \eqref{eq:stor_bound_all_pf} gives the same as for $\mathbf{x}^*$, so it is satisfied.
For \eqref{eq:stor_p_pf}, at $t = \tau$, the constraint is satisfied since $q_v^{\tau'} \leq q_v^{\tau}$. At $t=\kappa$ it is also satisfied since $q_v^{\tau'} \geq 0$.
All constraints are satisfied, so this new solution is feasible. The value of the objective function for this solution is the same since $d_{lt}$ and $p_{gt}$ are the same and the total energy discharged for the inter-storage is the same.
We have thus found another solution in which the quantity discharged in $\tau$ is smaller. We can repeat the same procedure until there is no quantity discharged at $\tau$.

\paragraph{Recursion}

We can repeat the following until there is no simultaneous charge of the intra-storage and discharge of the inter-storage:
\begin{enumerate}
    \item We consider $\tau$, for which $p_\tau\up{C,a*} > 0$ and $\sum_{v \in \mathcal{V}} p_{v\tau}\up{D,e*} > 0$. We have $q_v^\tau = p_{v\tau}\up{D,e*}$, $\forall v \in \mathcal{V}$, and  $q^\tau = \sum_{v \in \mathcal{V}} q_v^\tau$.
    \item We identify $\kappa$ such that $p_\kappa\up{C,a*} < 0$.
    \item We modify the solution. We identify $q^{\tau'} = \min \{q^{\tau}, -p_\kappa\up{C,a*}\}$ and $q_v^{\tau'}$, such that $q^{\tau'}= \sum_{v \in \mathcal{V}} q_v^{\tau'}$ and $0 \leq q_v^{\tau'} \leq q_v^{\tau}$, $\forall v \in \mathcal{V}$. For $t=\tau$, $p_\tau\up{C,a'} = p_\tau\up{C,a*} - q^{\tau'}$ and $p_{v\tau}\up{D,e'} = p_{v\tau}\up{D,e*} - q_v^{\tau'}$. For $t=\kappa$, $p_\kappa\up{C,a'} = p_\kappa\up{C,a*} + q^{\tau'}$ and $p_{v\kappa}\up{D,e'} = p_{v\kappa}\up{D,e*} + q_v^{\tau'}$, $\forall v \in \mathcal{V}$. 
    \item We update $q\up{\tau, new} = q\up{\tau, old} - q^{\tau'}$.
    \item If $q\up{\tau, new} > 0$, we go back to step 2 and identify a new $\kappa$. If $q\up{\tau, new} = 0$, we go to step 6.
    \item Check if there is another $t$ for which  $p_t\up{C,a*} > 0$ and $\sum_{v \in \mathcal{V}} p_{vt}\up{D,e*} > 0$. If so, it is the new $\tau$ and we go back to 1.
\end{enumerate}

We have shown that there is always an optimal solution in which there is no simultaneous charge and discharge, under the assumption that $S_v > 0$, $\forall v \in \mathcal{V}$, and how to obtain it.
